# Supplementary material for: Modular and On-demand Bias Mitigation with Attribute-Removal Subnetworks
Source: arXiv:2205.15171 source file (2023-06-04)
Supplement: Supplementary file 1 [file BACKUP-9-appendix.tex]

\begin{figure*}[h]
  \centering
  \includegraphics[width=0.95\linewidth]{figures/density.png}
  \caption{Modular Diff-Pruning 90\% vs. separate task-only and adversarial Diff-Pruning models 90\%: density per layer and module. Percentage values indicate the number of non-zero parameters in each layer averaged over 5 experiments. Top most and right most values show the totals for the respective layers and modules.}
  \label{fig:density}
\end{figure*}

\begin{table*}[t]
\centering
    \begin{tabular}{lSSSSSS}
        \toprule
        \multirow{2}{*}{} &
        \multicolumn{1}{c}{task acc} &
        \multicolumn{2}{c}{prot attr bac} \\
        &  {} & {gender} & {age} \\
        \midrule
        Finetuned & {$91.4 \pm 0.2$} & {$64.4 \pm 1.0$} & {$46.3 \pm 1.8$} \\
        Finetuned Adv & {$00.0 \pm 0.0$} & {$00.0 \pm 0.0$} & {$00.0 \pm 0.0$} \\
        \midrule
        Diff-Pruning 95\% & {$90.0 \pm 0.1$} & {$67.2 \pm 0.3$} & {$49.7 \pm 1.1$} \\
        Diff-Pruning 95\% Adv & {$00.0 \pm 0.0$} & {$00.0 \pm 0.0$} & {$00.0 \pm 0.0$} \\
        Diff-Pruning 90\% & {$91.0 \pm 0.2$} & {$67.0 \pm 0.4$} & {$49.5 \pm 0.7$} \\
        Diff-Pruning 90\% Adv & {$00.0 \pm 0.0$} & {$00.0 \pm 0.0$} & {$00.0 \pm 0.0$} \\
        \midrule
        Modular Finetuned Adv & {$00.0 \pm 0.0$} & {$00.0 \pm 0.0$} & {$00.0 \pm 0.0$} \\
        \midrule
        Modular Diff-Pruning 95\% Adv & {$00.0 \pm 0.0$} & {$00.0 \pm 0.0$} & {$00.0 \pm 0.0$} \\
        Modular Diff-Pruning 90\% Adv & {$00.0 \pm 0.0$} & {$00.0 \pm 0.0$} & {$00.0 \pm 0.0$} \\
        \bottomrule
    \end{tabular}
  \caption{pan16}
  \label{tab:results:pan16}
\end{table*}


\begin{table}[]
\centering
\begin{tabular}{lllccc}
\toprule
Model & Dataset & \multicolumn{1}{c}{Attribute} & task Acc & 1st attribute BAcc & 2nd attribute BAcc \\
Mini- Modular & Hate & Dielect & 0.799 ±0.006 & 0.854 ±0.016 & - \\
Mini- Modular & Pan16 & Gender Age & 0.915 ±0.003 & 0.609 ±0.013 & 0.413 ±0.011 \\
Mini- Modular & Pan16 & Gender & 0.916 ±0.001 & 0.609 ±0.004 & 0.4034 ±0.008 \\
Mini- Modular & Pan16 & Age & 0.915 ±0.002 & 0.608 ±0.006 & 0.416 ±0.007 \\
Mini- Modular & Bios & Gender & 0.814 ±0.002 & 0.588 ±0.008 & - \\  \midrule \hline 
Modular & Hate & Dielect & 0.808 ±0 & 0.847 ±0 & - \\
Modular & Pan16 & Gender Age & 0.938 ±0 & 0.537 ±0 & 0.299 ±0 \\
Modular & Pan16 & Gender & 0.936 ±0 & 0.591 ±0 & 0.354 ±0 \\
Modular & Pan16 & Age & 0.935 ±0 & 0.553 ±0 & 0.293 ±0 \\
Modular & Bios & Gender & 0.839 ±0 & 0.572 ±0 & - \\ \midrule \hline 
Baseline & Hate & Dielect & 0.819 ±0 & 0.877 ±0 & - \\
Baseline & Pan16 & Gender Age & 0.935 ±0 & 0.62 ±0 & 0.408 ±0 \\
Baseline & Pan16 & Gender & 0.937 ±0 & 0.623 ±0 & 0.43 ±0 \\
Baseline & Pan16 & Age & 0.938 ±0 & 0.62 ±0 & 0.427 ±0 \\
Baseline & Bios & Gender & 0.841 ±0 & 0.62 ±0 & - \\ \midrule \hline 
diff MMD & Hate & Dielect & 0.811 ±0 & 0.915 ±0 & - \\
diff MMD & Pan16 & Gender Age & ± & ± & ± \\
diff MMD & Pan16 & Gender & ± & ± & ± \\
diff MMD & Pan16 & Age & ± & ± & ± \\
diff MMD & Bios & Gender & ± & ± & - \\ \bottomrule
\end{tabular}
\end{table}
